# Supplementary material for: Twists and turns for metamaterials
Source: arXiv:1301.5960 ancillary file (2013-01-25)
Supplement: Supplementary file 1 [file supplement_v5.pdf]

# Supplemental materials: Twists and turns for metamaterials

Mingkai Liu, Yue Sun, David A. Powell, Ilya V. Shadrivov, Mikhail Lapine, Ross C. McPhedran, Yuri S. Kivshar

## THEORETICAL APPROACH

We model a pair of twisted SRRs, with radius  $r = 6$  mm and vertical spacing  $s = 2$  mm. The size of the slit in each ring can be described by the angle at which the gap is visible from the ring centre,  $\alpha_0 = 10^\circ$ . The elastic coupling is provided with a wire of radius  $a = 50$   $\mu$ m and of length  $d = 100$  mm, made from rubber with a shear modulus of  $G = 0.6$  MPa. The orientation of the gaps with respect to the incident electric field polarisation is described by the angle  $\Phi$  between the azimuth of the gap of the bottom ring as seen from the ring axis, and  $y$  axis. Changing  $\Phi$  generally leads to some difference in the coupling efficiency between the input plane wave and the eigenmodes, but does not cause any substantial qualitative difference such as the direction of EM torque, since it is a property governed by the symmetry of the mode profiles. Without a loss of generality, we have assumed  $\Phi = 0$  for the calculations presented in Fig. 2 of the article.

To capture the essential characteristics of the resonances and the optomechanical properties of the structure, we approximate the SRR as an infinitely thin line current with a sinusoidal distribution in the azimuthal direction. In Eq. (1) of the article, the effective voltages on each SRR due to the external field  $\mathbf{E}_{\text{ext}}$  and  $\mathbf{B}_{\text{ext}}$  are given by

$$\mathcal{E}_1 = -\mathbf{E}_{\text{ext}} \cdot \mathbf{l}_e \cdot e^{jk_0 a_E \cos \Phi} + j\omega \mathbf{B}_{\text{ext}} \cdot \mathbf{u}_e \cdot e^{jk_0 a_M \cos \Phi} \quad (1)$$

and

$$\mathcal{E}_2 = -\mathbf{E}_{\text{ext}} \cdot \mathbf{l}_e \cdot e^{jk_0 a_E \cos(\Phi + \theta)} + j\omega \mathbf{B}_{\text{ext}} \cdot \mathbf{u}_e \cdot e^{jk_0 a_M \cos(\Phi + \theta)} \quad (2)$$

The normalised electric dipole moment is  $\mathbf{l}_e(\theta, \Phi) = \int_V q(\mathbf{r}) \mathbf{r} dV$ , and  $\mathbf{u}_e(\theta, \Phi) = \frac{1}{2} \int_V \mathbf{r} \times \mathbf{j}(\mathbf{r}) dV$  is the normalised magnetic dipole moment.

We define the effective central positions of the electric and magnetic dipoles

$$a_E = \frac{\int_V [q(\mathbf{r}_1) \mathbf{r}_1 \cdot \hat{\mathbf{x}}] (\mathbf{r}_1 \cdot \hat{\mathbf{y}}) dV_1}{\left| \int_V q(\mathbf{r}_1) \mathbf{r}_1 dV_1 \right|} \quad (3)$$

$$a_M = \frac{\int_V [\mathbf{r}_1 \times \mathbf{j}(\mathbf{r}_1) \cdot \hat{\mathbf{z}}] (\mathbf{r}_1 \cdot \hat{\mathbf{y}}) dV_1}{\left| \int_V \mathbf{r}_1 \times \mathbf{j}(\mathbf{r}_1) dV_1 \right|} \quad (4)$$

similar to the definition of centre of mass, and they are calculated based on the charge and current distributions of the lower SRR when  $\Phi = 0$ . The phase terms of the effective voltages describe the phase retardation experienced by the SRRs in the direction of wave propagation.

$F_s = 1/C_s - \omega^2 L_s$  and  $F_m = 1/C_m - \omega^2 L_m$  are the self and mutual impedance terms, where the effective capacitances  $C$  and inductances  $L$  can be calculated from the modal current  $\mathbf{j}(\mathbf{r})$  and charge  $q(\mathbf{r})$  distributions (see Ref. 20).

Next we present the expressions for the internal (generated by the near-field interaction between SRRs) and external (generated by the incident electromagnetic wave) components of the electromagnetic torque. Due to the structural symmetry, the magnetic part does not contribute to the torque in the  $z$  direction. The time-averaged external torque can then be written in a compact form:

$$\mathbf{M}_{\text{ext},2} = \frac{1}{2} \text{Re} \left[ \int_{V_2} \rho^*(\mathbf{r}_2) \mathbf{r}_2 \times \mathbf{E}_{\text{ext}} dV_2 \right] = -\frac{1}{2} \text{Re} \left[ Q_2^*(\omega, \Phi) e^{jk_0 a_E \cos(\Phi + \theta)} \right] \mathbf{E}_{\text{ext}} \cdot \mathbf{l}_e \sin(\Phi + \theta) \cdot \hat{\mathbf{z}} \quad (5)$$

while the internal torque can be expressed as

$$\mathbf{M}_{\text{int},2} = \frac{1}{2} \text{Re} \left[ \int_{V_2} \rho^*(\mathbf{r}_2) \mathbf{r}_2 \times \mathbf{E}_{\text{int}}(\mathbf{r}_2) dV_2 \right] \quad (6)$$

with

$$\mathbf{E}_{\text{int}}(\mathbf{r}_2) = -\nabla \phi(\mathbf{r}_2) - \frac{\partial}{\partial t} \mathbf{A}(\mathbf{r}_2) = - \int_{V_1} \nabla \frac{\rho(\mathbf{r}_1) e^{jk|\mathbf{r}_2 - \mathbf{r}_1|}}{4\pi\epsilon_0 |\mathbf{r}_2 - \mathbf{r}_1|} + \frac{\partial}{\partial t} \frac{\mathbf{J}(\mathbf{r}_1) e^{jk|\mathbf{r}_2 - \mathbf{r}_1|}}{4\pi c^2 \epsilon_0 |\mathbf{r}_2 - \mathbf{r}_1|} dV_1 \quad (7)$$

Finally, we arrive at

$$\mathbf{M}_{\text{int},2} = \frac{1}{2} \text{Re} \left\{ \frac{Q_1(\omega) Q_2^*(\omega)}{4\pi\epsilon_0} \int \int \frac{q^*(\mathbf{r}_2) e^{jk|\mathbf{r}_1 - \mathbf{r}_2|}}{|\mathbf{r}_1 - \mathbf{r}_2|} \left[ \frac{1 - jk|\mathbf{r}_1 - \mathbf{r}_2|}{|\mathbf{r}_1 - \mathbf{r}_2|^2} q(\mathbf{r}_1) \mathbf{r}_1 \times \mathbf{r}_2 + k^2 \mathbf{r}_2 \times \mathbf{j}(\mathbf{r}_1) \right] dV_1 dV_2 \right\} \quad (8)$$

For a cylindrical wire that can be used to suspend the rotatable SRR, the restoring torque can be estimated as  $M_R = -\pi a^4 G(\theta - \theta_0)/(2d)$ , where  $a$  and  $d$  are the radius and the length of the wire, respectively.  $G$  is the shear modulus and  $\theta_0$  is the initial twist angle of the structure. A series of equilibrium twist angles can be found by solving the nonlinear equation  $M_{EM}(\theta, P_I) + M_R(\theta, \theta_0) = 0$ .

### COMPARISON OF ARRAY AND WAVEGUIDE GEOMETRIES

Due to the formation of image currents within the waveguide walls, a single meta-atom within a waveguide has virtual neighbours. Just as in an array, there will be near-field interaction with these virtual neighbours, with some alteration due to the mirror reflections. This suggests that the waveguide system is strongly analogous to an array, at least for relatively dilute lattice spacing. To verify this, we numerically model the electromagnetic torque of the system for both the waveguide and array geometries. The field distribution is calculated numerically using CST Microwave Studio, and the EM torque exerted on the top SRR is calculated with the Maxwell stress tensor. As shown in Fig. S1, the qualitative agreement between the two is very good.

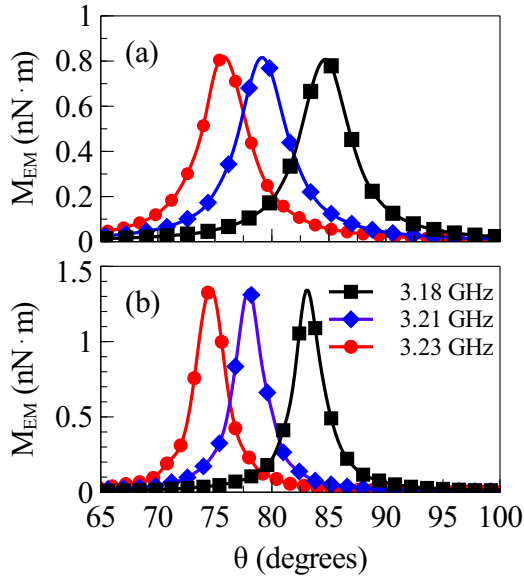

FIG. S1. Mutual EM torque as a function of twist angle under different pump frequencies. (a) single chiral meta-atom in waveguide, (b) periodic array of chiral meta-atoms, with periodicity 45 mm in the lateral direction and one layer in the propagating direction of EM wave. The torques shown correspond to a 1W power pumped into the waveguide or one unit cell.

### EXPERIMENTAL MEASUREMENTS AND COMPARISON WITH NUMERICAL RESULTS

Since the mechanism of nonlinear response is the dynamic coupling between electromagnetic and elastic properties, the experimental setup exhibits the same physics as the conceptual schematic. In the experiment, it was not necessary to fix the bottom end of the wire to the substrate, because the maximum forces emerging in the lateral directions ( $\sim 0.1 \mu\text{N}$  according to our calculations) can only produce a negligible swing angle ( $0.056^\circ$ ) since they are much smaller than the weight of the sample ( $\sim 980 \mu\text{N}$ ). The calculated torque is a Lorentz-like function and the maximum is around 0.8 nNm. The maximum attractive force between the two SRRs is around  $2 \mu\text{N}$ , which leads to a negligible elongation of the wire ( $0.012\%$ ); while the force in the lateral direction is around  $0.1 \mu\text{N}$ , about 1000 times smaller than the gravitational force exerted on the sample, and thus it only gives rise to a tiny swing angle ( $0.056^\circ$ ).

All the key results of the experimental measurements are shown in Figure 4 (a), (c) and (e) of the paper. For completeness, Fig. S2 depicts the measured transmission coefficients  $|S_{21}|$  under different pump frequencies and powers with a 1 dB step between the curves.

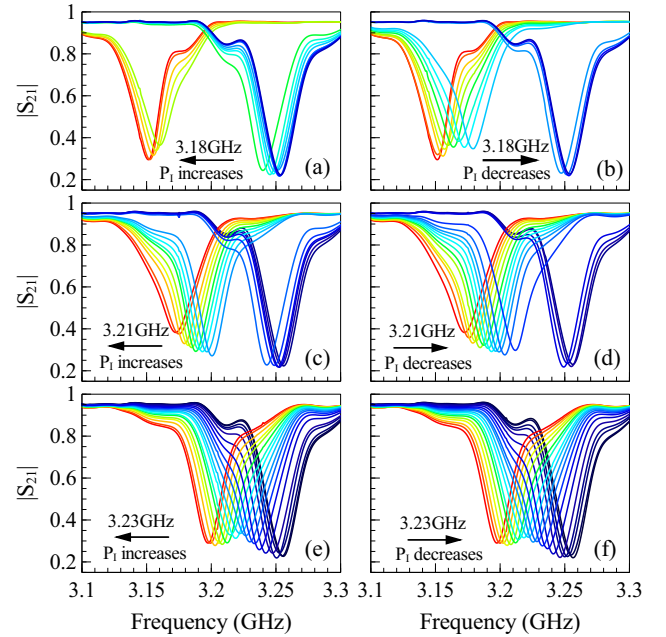

FIG. S2. Experimental transmission coefficients  $|S_{21}|$  for different pump frequencies and powers. The initial resonance locates around 3.256 GHz and the pump power is swept in 1 dB steps. (a) and (b) pump at 3.18 GHz, power changes from 15.2 dBm to 27.2 dBm; (c) and (d) pump at 3.21 GHz, power changes from 12.2 dBm to 27.2 dBm; (d) and (e) pump at 3.23 GHz, power changes from 15.2 dBm to 27.2 dBm.

Finally, to verify that our numerical simulations are comparable with our experimental system, we have per-

formed a numerical calculation for the exact experimental configuration. Following the procedure described in the theoretical part, we numerically calculate the EM torque and find a series of stable twist angles for different pump power. In Fig. S3, we have reproduced the experimental results from Figure 4 in the manuscript. In addition, we show an exactly corresponding numerical simulation. In general this agreement is quite good, thus confirming that our numerical model has reproduced the experimental configuration with acceptable accuracy.

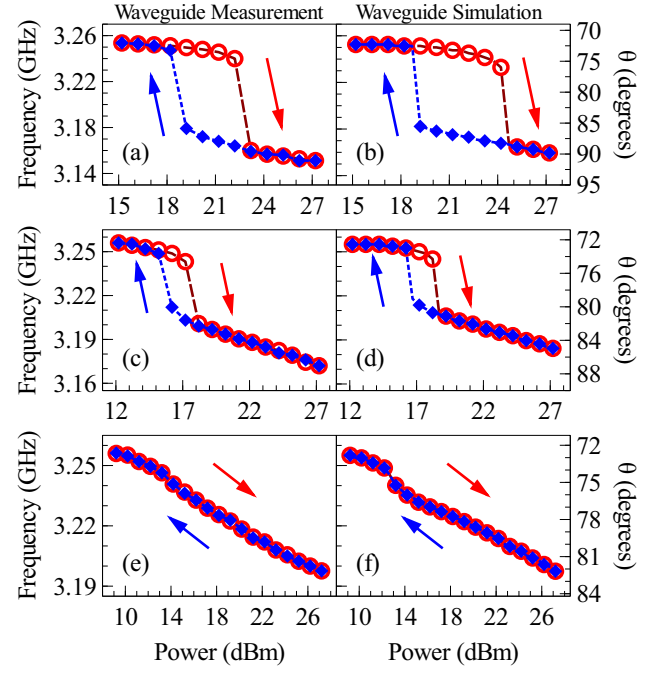

FIG. S3. Comparison of experimentally (a), (c), (e) and numerically (b), (d), (f) calculated resonant frequency sweeps for identical geometry. The corresponding stable twist angles are shown on the right axes.
